# Supplementary material for: Orthogonal Gradient Boosting for Simpler Additive Rule Ensembles
Source: arXiv:2402.15691 source file (2024-02-24)
Supplement: Supplementary file 1 [file SI_table.tex]

\begin{table*}
\addtocounter{table}{1}
\caption{Comparison of Test Risks of Gradient Sum(S), Gradient boosting (G), XGBoost (X) and FCOGB (O) for benchmark datasets of classification (upper), regression (middle) and Poisson regression problems (lower). The lowest training and test risks for each dataset are bolded. The red colours indicate the COB approach using either greedy search or branch-and-bound search have lower risks than all the other methods.}
\label{tb:comparison_test}
\vskip 0.05in
% \hskip 0.05in
\begin{center}
\begin{small}
\begin{sc}
\begin{tabular}{l@{\hskip 0.05in}c@{\hskip 0.03in}c@{\hskip 0.03in}c@{\hskip 0.05in}c@{\hskip 0.05in}c@{\hskip 0.05in}c@{\hskip 0.05in}c@{\hskip 0.05in}c@{\hskip 0.05in}c@{\hskip 0.05in}c@{\hskip 0.05in}c@{\hskip 0.05in}c@{\hskip 0.05in}c@{\hskip 0.05in}c@{\hskip 0.05in}c@{\hskip 0.05in}c@{\hskip 0.05in}c@{\hskip 0.05in}c@{\hskip 0.05in}c@{\hskip 0.05in}c@{\hskip 0.05in}c@{\hskip 0.05in}c@{\hskip 0.05in}r}
% \begin{tabular}{lcccccccccccccccr}
\toprule

\multirow{2}{*}{dataset} & \multirow{2}{*}{feat} & \multirow{2}{*}{row} & \multirow{2}{*}{$\bar{\Tilde{R}}_\mathrm{O}$} & \multicolumn{5}{c}{FCOGB vs. GS} & \multicolumn{5}{c}{FCOGB vs. GB} & \multicolumn{5}{c}{FCOGB vs XGBoost} \\
 &  &  &  & \multicolumn{2}{c}{$\Delta_\mathrm{SO}^\mathrm{bc}$} & \multicolumn{1}{c}{$\bar{\Delta}_\mathrm{SO}$} & \multicolumn{2}{c}{$\Delta_\mathrm{SO}^\mathrm{wc}$} & \multicolumn{2}{c}{$\Delta_\mathrm{GO}^\mathrm{bc}$} & $\bar{\Delta}_\mathrm{GO}$ & \multicolumn{2}{c}{$\Delta_\mathrm{GO}^\mathrm{wc}$} & \multicolumn{2}{c}{$\Delta_\mathrm{XO}^\mathrm{bc}$} & $\bar{\Delta}_\mathrm{XO}$ & \multicolumn{2}{c}{$\Delta_\mathrm{XO}^\mathrm{wc}$} \\

\midrule
titanic & 7 & 1043 & .712 & .074 & (17.6) & .035 & .000 & (2.4) & .147 & (2.4) & .025 & -.025 & (28.2) & .147 & (2.4) & .022 & -.015 & (4.4) \\
tic-tac-toe & 27 & 958 & .751 & .174 & (23.6) & .101 & -.058 & (1.4) & .111 & (6.2) & .060 & .000 & (2.4) & .089 & (16.8) & .030 & -.013 & (28.4) \\
iris & 4 & 150 & .552 & .141 & (5.8) & -.089 & -.180 & (7.2) & .149 & (2.4) & -.083 & -.294 & (5) & .149 & (2.4) & -.058 & -.147 & (25.8) \\
breast & 30 & 569 & .352 & .024 & (7.8) & -.055 & -.229 & (7) & .009 & (7.8) & -.011 & -.026 & (26) & .100 & (7.8) & .031 & -.006 & (20.2) \\
wine & 13 & 178 & .368 & .314 & (2.4) & .020 & -.270 & (5.8) & .409 & (6) & .135 & .003 & (4) & .433 & (6) & .090 & -.043 & (27) \\
ibm hr & 32 & 1470 & .217 & .019 & (6.2) & .003 & -.005 & (8.2) & .034 & (15.4) & .004 & .000 & (1.4) & .065 & (4) & .012 & .004 & (1.4) \\
telco churn & 18 & 7043 & .688 & .058 & (2.4) & .005 & -.159 & (1.4) & .037 & (23.4) & .019 & -.032 & (8.2) & .017 & (9.4) & .006 & -.009 & (12.4) \\
gender & 20 & 3168 & .999 & .003 & (2.4) & .001 & .002 & (3.2) & .000 & (4.2) & .000 & .000 & (2.4) & .003 & (11.4) & .001 & .000 & (2.4) \\
banknote & 4 & 1372 & .355 & .142 & (19.6) & .055 & -.075 & (8.2) & .133 & (19.6) & .024 & -.079 & (9.4) & .120 & (19.6) & .049 & -.049 & (9.4) \\
liver & 6 & 345 & .999 & -.012 & (3.8) & -.093 & -.195 & (29.8) & .057 & (3.8) & -.024 & -.067 & (15.4) & .057 & (3.8) & -.066 & -.164 & (29.4) \\
magic & 10 & 19020 & .710 & .056 & (8.2) & .018 & -.037 & (4.2) & .018 & (15.4) & .007 & .000 & (5.2) & .017 & (18.4) & .007 & -.003 & (25.4) \\
adult & 11 & 30162 & .619 & .146 & (2.4) & .007 & -.191 & (1.4) & .059 & (10.4) & .018 & .000 & (2.4) & .058 & (4.2) & .011 & .004 & (20.4) \\
digits5 & 64 & 3915 & .381 & .030 & (4.2) & .014 & -.008 & (3.2) & .009 & (4.2) & -.031 & -.058 & (19.4) & .070 & (4.2) & -.004 & -.034 & (19.4) \\
\midrule
insurance & 6 & 1338 & .163 & .104 & (7.2) & .017 & -.567 & (1.4) & .172 & (4.2) & .018 & -.011 & (5.2) & .172 & (4.2) & .020 & -.011 & (5.2) \\
friedman1 & 10 & 2000 & .083 & .013 & (4) & -.002 & -.012 & (3.2) & .025 & (4) & .006 & .000 & (1.4) & .025 & (4) & .005 & .000 & (1.4) \\
friedman2 & 4 & 10000 & .149 & .165 & (3.2) & -.021 & -.612 & (1.4) & .084 & (10.4) & .019 & -.068 & (5.2) & .080 & (8.2) & .016 & -.068 & (5.2) \\
friedman3 & 4 & 5000 & .060 & .009 & (4.6) & .003 & -.012 & (4) & .021 & (4.6) & .002 & .000 & (1.4) & .021 & (4.6) & .002 & .000 & (1.4) \\
wage & 5 & 1379 & .419 & .017 & (6.6) & -.021 & -.048 & (4.6) & .065 & (6.6) & .000 & -.027 & (18.2) & .065 & (6.6) & -.002 & -.014 & (21.4) \\
demographics & 13 & 6876 & .229 & .011 & (5.2) & .003 & .000 & (1.4) & .007 & (3.2) & .002 & .000 & (1.4) & .007 & (3.2) & .002 & .000 & (1.4) \\
gdp & 1 & 35 & .038 & .003 & (3.2) & .000 & -.001 & (5.2) & .003 & (3.2) & .000 & -.001 & (5.2) & .003 & (3.2) & .000 & -.001 & (5.2) \\
used cars & 4 & 1770 & .198 & .178 & (3.2) & -.019 & -.549 & (1.4) & .113 & (14) & .055 & .000 & (3.2) & .089 & (8.8) & .035 & .000 & (3.2) \\
diabetes & 10 & 442 & .169 & .026 & (4.4) & -.004 & -.033 & (3.4) & .058 & (4.4) & -.002 & -.011 & (29.8) & .058 & (4.4) & .002 & -.008 & (29.4) \\
boston & 13 & 506 & .097 & .019 & (4.4) & -.001 & -.025 & (3.8) & .044 & (4.4) & .006 & -.011 & (8.6) & .044 & (4.4) & .006 & -.011 & (9.2) \\
world happiness & 8 & 315 & .051 & .010 & (5.2) & -.003 & -.012 & (3.8) & .013 & (5.2) & .002 & -.010 & (4.4) & .023 & (5.2) & .002 & -.001 & (23.6) \\
life expectancy & 21 & 1649 & .041 & .003 & (4.2) & .000 & -.001 & (8.2) & .007 & (4.2) & .001 & .000 & (20.4) & .007 & (4.2) & .001 & -.001 & (26.4) \\
mobile prices & 20 & 2000 & .168 & .168 & (2.4) & -.008 & -.648 & (1.4) & .058 & (3.2) & .002 & -.004 & (8.2) & .058 & (3.2) & .004 & .000 & (4.2) \\
suicide rate & 5 & 27820 & .534 & .081 & (2.4) & .016 & -.333 & (1.4) & .018 & (13.4) & .008 & .000 & (2.4) & .024 & (11.4) & .009 & .000 & (2.4) \\
video games & 6 & 16327 & .723 & .000 & (4.2) & .000 & .000 & (3.2) & .000 & (10.4) & .000 & .000 & (3.2) & .000 & (10.4) & .000 & .000 & (3.2) \\
red wine & 11 & 1599 & .048 & .003 & (4.2) & .000 & -.002 & (3.2) & .004 & (4.2) & .001 & .000 & (1.4) & .004 & (4.2) & .001 & .000 & (7.4) \\
\midrule
covid vic & 4 & 85 & .185 & .068 & (3) & .030 & -.062 & (10) & .103 & (10.6) & -.005 & -.692 & (2.8) & 3.448 & (3) & .418 & .002 & (25.8) \\
covid & 2 & 225 & .515 & .071 & (6.8) & -.037 & -.399 & (2) & .279 & (3.8) & .025 & -.003 & (27) & 25.66 & (6.8) & 5.388 & .290 & (26.8) \\
bicycle & 4 & 122 & .505 & .213 & (7.8) & -.021 & -.333 & (3.4) & .054 & (4.6) & -.035 & -.337 & (4) & .011 & (7.8) & -.025 & -.061 & (22.2) \\
ships & 4 & 34 & .338 & .076 & (3.2) & -.089 & -.498 & (2.4) & .160 & (11) & .015 & -.066 & (23.2) & 993.4 & (3.2) & 181.3 & .605 & (29.6) \\
smoking & 2 & 36 & .216 & -.017 & (16.6) & -.046 & -.189 & (6.6) & .075 & (10.2) & .029 & -.043 & (4.2) & .950 & (2.4) & .124 & .035 & (14.2) \\

\bottomrule
\end{tabular}
\end{sc}
\end{small}
\end{center}
\vskip -0.1in
\end{table*}
