# Supplementary material for: Orthogonal Gradient Boosting for Simpler Additive Rule Ensembles
Source: arXiv:2402.15691 source file (2024-02-24)
Supplement: Supplementary file 2 [file SI_table_Greedy_time.tex]

\begin{table*}[]
\caption{Comparison of average normalised risks and computation times of Gradient Sum (GS), Gradient Boosting (GB), XGBoost, FCOGB using Branch-and-bound (BB FCOGB) and FCOGB using Greedy search (Greedy FCOGB)}
\label{tb:comparison_greedy}
\begin{center}
\begin{small}
\begin{sc}
\begin{tabular}{l@{\hskip 0.03in}c@{\hskip 0.03in}c@{\hskip 0.03in}c@{\hskip 0.03in}c@{\hskip 0.03in}c@{\hskip 0.03in}c@{\hskip 0.03in}c@{\hskip 0.03in}c@{\hskip 0.03in}c@{\hskip 0.03in}c@{\hskip 0.03in}c@{\hskip 0.03in}c@{\hskip 0.03in}c}

\hline
\multicolumn{1}{c}{\multirow{2}{*}{dataset}} & \multicolumn{1}{c}{\multirow{2}{*}{$d$}} & \multicolumn{1}{c}{\multirow{2}{*}{$n$}} & \multicolumn{5}{c}{Average normalised risks} & \multicolumn{5}{c}{Computation times} \\
\multicolumn{1}{c}{} & \multicolumn{1}{c}{} & \multicolumn{1}{c}{} & GS & GB & XGB & \begin{tabular}[c]{@{}l@{}}BB \\ FCOGB\end{tabular} & \begin{tabular}[c]{@{}l@{}}Greedy \\ FCOGB\end{tabular} & GS & GB & XGB & \begin{tabular}[c]{@{}l@{}}BB \\ FCOGB\end{tabular} & \begin{tabular}[c]{@{}l@{}}Greedy \\ FCOGB\end{tabular} \\ \hline
titanic & 7 & 1043 & .702 & .675 & .694 & \textbf{.658} & .679 & 1.660 & 20.87 & 26.81 & 26.44 & 1.799 \\
tic-tac-toe & 27 & 958 & .805 & .693 & .744 & \textbf{.656} & .735 & 5.570 & 29.29 & 23.06 & 47.68 & 2.012 \\
iris & 4 & 150 & .359 & .344 & .379 & .317 & \textbf{.295} & .785 & 2.010 & 2.075 & 2.090 & .441 \\
breast & 30 & 569 & \textbf{.347} & .361 & .391 & .358 & .359 & 8.505 & 116.2 & 177.8 & 257.3 & 3.818 \\
wine & 13 & 178 & .286 & .303 & .353 & \textbf{.241} & .305 & 2.015 & 7.713 & 1.151 & 30.09 & .935 \\
ibm hr & 32 & 1470 & .592 & .215 & .596 & \textbf{.212} & .578 & 15.67 & 7.488 & 20.25 & 11.44 & 5.078 \\
telco churn & 18 & 7043 & .707 & .714 & .703 & .695 & \textbf{.694} & 22.45 & 5266 & 5190 & 5343 & 28.89 \\
gender & 20 & 3168 & .997 & .997 & .997 & \textbf{.997} & .997 & 6.543 & 42.66 & 32.38 & 28.47 & 7.031 \\
banknote & 4 & 1372 & .394 & .354 & .406 & \textbf{.337} & .356 & 6.492 & 10.08 & 13.83 & 6.991 & 3.103 \\
liver & 6 & 345 & .855 & \textbf{.833} & .860 & .837 & .862 & 2.015 & 145.2 & 301.4 & 234.5 & 1.364 \\
magic & 10 & 19020 & .744 & \textbf{.729} & .737 & .731 & .733 & 73.11 & 71.10 & 194.2 & 138.9 & 78.03 \\
adult & 11 & 30162 & .620 & .626 & .614 & .608 & \textbf{.600} & 100.9 & 392.0 & 381.7 & 347.5 & 156.6 \\
digits5 & 64 & 3915 & .413 & .385 & .401 & .393 & \textbf{.364} & 60.38 & 110.7 & 37.98 & 125.8 & 38.84 \\ \hline
insurance & 6 & 1338 & .193 & .192 & .190 & \textbf{.166} & .169 & 10.90 & 19.50 & 37.62 & 28.48 & 3.110 \\
friedman1 & 10 & 2000 & .096 & .084 & .102 & \textbf{.080} & .093 & 2.795 & 5.347 & 12.38 & 6.220 & 1.242 \\
friedman2 & 4 & 10000 & .188 & .165 & .252 & \textbf{.149} & .223 & 22.89 & 19.723 & 30.60 & 12.65 & 5.716 \\
friedman3 & 4 & 5000 & .061 & .060 & .060 & \textbf{.057} & .057 & 8.313 & 12.766 & 27.42 & 12.37 & 2.836 \\
wage & 5 & 1379 & .396 & .394 & .401 & \textbf{.381} & .386 & 9.077 & 21.263 & 29.60 & 20.64 & 3.158 \\
demographics & 13 & 6876 & .229 & .227 & .227 & \textbf{.225} & .225 & 36.37 & 21.707 & 49.56 & 30.39 & 14.56 \\
gdp & 1 & 35 & .038 & .038 & .038 & \textbf{.037} & .037 & .086 & .263 & .429 & .351 & .094 \\
used cars & 4 & 1770 & \textbf{.171} & .224 & .243 & .191 & .190 & 13.23 & 17.40 & 34.90 & 12.46 & 4.121 \\
diabetes & 10 & 442 & .157 & .160 & .159 & .153 & \textbf{.151} & 2.598 & 5.813 & 8.926 & 7.529 & 1.567 \\
boston & 13 & 506 & .111 & .110 & .112 & \textbf{.103} & .104 & 3.942 & 8.186 & 16.226 & 8.591 & 1.543 \\
happiness & 8 & 315 & .047 & .049 & .048 & .047 & .045 & .561 & 13.79 & 26.37 & 24.02 & .609 \\
life expect. & 21 & 1649 & .040 & .041 & .041 & \textbf{.040} & .040 & 20.28 & 55.46 & 144.6 & 150.6 & 7.145 \\
mobile prices & 20 & 2000 & \textbf{.157} & .166 & .166 & .163 & .162 & 21.67 & 775.4 & 1736 & 1101 & 7.738 \\
suicide rate & 5 & 27820 & .578 & .562 & .562 & \textbf{.553} & .562 & 74.23 & 161.1 & 45.59 & 178.8 & 95.55 \\
videogame & 6 & 16327 & .954 & .954 & .954 & \textbf{.954} & .954 & 20.21 & 58.91 & 14.21 & 37.72 & 18.16 \\
red wine & 11 & 1599 & .048 & .048 & .049 & \textbf{.048} & .048 & 3.736 & 30.03 & 17.72 & 37.25 & 3.924 \\ \hline
covid vic & 4 & 85 & .202 & .192 & .540 & .178 & \textbf{.168} & .580 & .729 & 1.502 & .587 & .247 \\
covid & 2 & 225 & \textbf{.386} & .419 & 4.133 & .408 & .422 & 1.032 & 1.026 & 2.153 & .832 & .420 \\
bicycle & 4 & 122 & .437 & .405 & .416 & .401 & \textbf{.397} & .792 & 1.897 & 3.536 & 1.768 & .421 \\
ships & 4 & 34 & \textbf{.212} & .255 & 129.2 & .223 & .203 & .265 & .367 & .597 & .362 & .141 \\
smoking & 2 & 36 & .171 & .155 & .260 & \textbf{.142} & .145 & .191 & .341 & .484 & .205 & .104 \\ \hline

\end{tabular}
 \end{sc}
\end{small}
\end{center}
\end{table*}
