# Supplementary material for: Orthogonal Gradient Boosting for Simpler Additive Rule Ensembles
Source: arXiv:2402.15691 source file (2024-02-24)
Supplement: Supplementary file 4 [file SI_table_scores.tex]

\begin{table}
\addtocounter{figure}{1}
\caption{Comparison of the area under the score / cognitive complexity curve of SIRUS, Gradient Sum(GS), Gradient boosting (GB), XGBoost (XGB) and FCOGB for benchmark datasets of classification (upper), regression (middle) and Poisson regression problems (lower).}
\label{tb:comparison_score}

\begin{tabular}{l@{\hskip 0.03in}c@{\hskip 0.03in}c@{\hskip 0.03in}c@{\hskip 0.03in}c@{\hskip 0.03in}c@{\hskip 0.03in}c@{\hskip 0.03in}c@{\hskip 0.03in}c@{\hskip 0.03in}c@{\hskip 0.03in}c@{\hskip 0.03in}c@{\hskip 0.03in}c@{\hskip 0.03in}}
 \toprule
 &  &  & \multicolumn{5}{c}{Training Scores / CC AUC} & \multicolumn{5}{c}{Testing Scores / CC AUC} \\

\multirow{-2}{*}{Dataset} & \multirow{-2}{*}{$d$} & \multirow{-2}{*}{$n$} & SIRUS & GS & GB & XGB & FCOGB & SIRUS & GS & GB & XGB & FCOGB \\ \hline
titanic & 7 & 1043 & .783 & .858 & .846 & .856 & \textbf{.866} & .803 & \textbf{.826} & .805 & .800 & .816 \\
tic-tac-toe & 27 & 958 & .677 & .783 & .878 & .888 & \textbf{.897} & .669 & .729 & .822 & .856 & \textbf{.867} \\
iris & 4 & 150 & .854 & .962 & .960 & .952 & \textbf{.964} & .781 & \textbf{.941} & .909 & .925 & .913 \\
breast & 30 & 569 & .930 & \textbf{.965} & .961 & .964 & .960 & .890 & \textbf{.964} & .935 & .946 & .951 \\
wine & 13 & 178 & .929 & \textbf{.975} & .954 & .966 & .974 & .912 & .962 & .905 & .931 & \textbf{.976} \\
ibm hr & 32 & 1470 & .700 & .426 & .628 & .690 & \textbf{.731} & \textbf{.696} & .417 & .591 & .634 & .679 \\
telco churn & 18 & 7043 & .756 & .796 & .790 & .787 & \textbf{.798} & .776 & \textbf{.808} & .794 & .795 & .798 \\
gender & 20 & 3168 & \textbf{.925} & .243 & .288 & .288 & .202 & \textbf{.926} & .240 & .285 & .285 & .200 \\
banknote & 4 & 1372 & .874 & .968 & .965 & \textbf{.969} & .967 & .870 & .967 & .965 & .967 & \textbf{.967} \\
liver & 6 & 345 & .701 & .812 & .792 & .807 & \textbf{.812} & \textbf{.699} & .687 & .650 & .622 & .576 \\
magic & 10 & 19020 & .602 & .778 & .805 & .806 & \textbf{.806} & .605 & .788 & .812 & \textbf{.814} & .813 \\
adult & 11 & 30162 & .726 & .731 & .838 & .842 & \textbf{.847} & .722 & .725 & .828 & .832 & \textbf{.837} \\
digits5 & 64 & 3915 & .423 & .465 & .732 & .741 & \textbf{.828} & .360 & .451 & .715 & .728 & \textbf{.797} \\ \hline
insurance & 6 & 1338 & .706 & .682 & .794 & .795 & \textbf{.824} & .633 & .683 & .782 & .770 & \textbf{.791} \\
friedman1 & 10 & 2000 & \textbf{.637} & .458 & .556 & .579 & .605 & \textbf{.633} & .409 & .431 & .430 & .458 \\
friedman2 & 4 & 10000 & .523 & .721 & .867 & .873 & \textbf{.894} & .536 & .721 & .868 & .873 & \textbf{.893} \\
friedman3 & 4 & 5000 & .590 & .539 & .616 & .630 & \textbf{.657} & .547 & .528 & .563 & .552 & \textbf{.571} \\
wage & 5 & 1379 & .217 & .308 & .334 & .358 & \textbf{.383} & .182 & \textbf{.244} & .207 & .200 & .180 \\
demographics & 13 & 6876 & \textbf{.367} & .103 & .168 & .187 & .203 & \textbf{.389} & .102 & .160 & .174 & .187 \\
gdp & 1 & 35 & \textbf{.663} & .469 & .444 & .480 & .513 & \textbf{.616} & .434 & .403 & .437 & .461 \\
used cars & 4 & 1770 & .679 & .766 & .820 & .823 & \textbf{.848} & .654 & .753 & .810 & .810 & \textbf{.834} \\
diabetes & 10 & 442 & .448 & .386 & .478 & .491 & \textbf{.520} & \textbf{.377} & .324 & .348 & .318 & .270 \\
boston & 13 & 506 & .642 & .493 & .595 & .616 & \textbf{.642} & \textbf{.590} & .441 & .425 & .430 & .426 \\
happiness & 8 & 315 & .077 & .789 & .804 & .802 & \textbf{.838} & .032 & \textbf{.675} & .541 & .524 & .572 \\
life expect. & 21 & 1649 & .662 & .622 & .671 & .685 & \textbf{.717} & \textbf{.641} & .558 & .603 & .606 & .613 \\
mobile prices & 20 & 2000 & .696 & .618 & .720 & .723 & \textbf{.726} & \textbf{.711} & .596 & .684 & .671 & .676 \\
suicide rate & 5 & 27820 & \textbf{.287} & .125 & .147 & .153 & .203 & \textbf{.289} & .127 & .149 & .154 & .204 \\
videogame & 6 & 16327 & \textbf{.015} & .001 & .001 & .001 & .001 & \textbf{.016} & .001 & .001 & .001 & .001 \\
red wine & 11 & 1599 & .251 & .242 & .285 & .304 & \textbf{.317} & .177 & .248 & .243 & .237 & \textbf{.262} \\ \hline
covid vic & 4 & 85 & NA & .678 & \textbf{.845} & NA & .827 & NA & .691 & \textbf{.865} & NA & .835 \\
covid & 2 & 225 & NA & .412 & .476 & {\color[HTML]{013300} NA} & \textbf{.514} & NA & .203 & \textbf{.205} & {\color[HTML]{333333} NA} & .200 \\
bicycle & 4 & 122 & NA & .707 & .778 & .789 & \textbf{.810} & NA & .623 & .596 & \textbf{.630} & .591 \\
ships & 4 & 34 & NA & .866 & .925 & {\color[HTML]{013300} NA} & \textbf{.946} & NA & .484 & \textbf{.514} & {\color[HTML]{333333} NA} & NA \\
smoking & 2 & 36 & NA & .677 & .943 & .829 & \textbf{.957} & NA & .607 & .756 & .591 & \textbf{.801}\\
\bottomrule
\end{tabular}
\end{table}
